# Supplementary material for: Fine-tuning Pre-trained Language Models for Few-shot Intent Detection: Supervised Pre-training and Isotropization
Source: arXiv:2205.07208 source file (2024-09-15)
Supplement: Supplementary file 1 [file appendix.tex]

\section{Appendix}
\label{sec:appendix}
\subsection{Additional Results of Pilot Study}
To show the impact of fine-tuning on isotropy, we visualize the covariance matrix of the feature space in Fig.~\ref{figure_fineTune_affect_covarianceMatrix}. It is found that after fine-tuning,  the covariance is strengthened in general. Pefect isotropy requires uniform variance and zero covariance, and thus the changes in the covariance matrix agrees with the isotropy measurement presented in Table~\ref{table: pilot, fine-tune affects isotropy.}.
\input{figures/figure_fine-tune_affect_covarianceMatrix}
